# Supplementary material for: Peculiar modules for 4-ended tangles
Source: arXiv:1712.05050 ancillary file (2019-07-08)
Supplement: Supplementary file 1 [file Manual_PQM.pdf]

# MANUAL FOR PQM.M

CLAUDIUS ZIBROWIUS

version 1.0, written in Mathematica 11.3

The Mathematica package `PQM.m` [5] provides a tool for calculating the immersed curve invariant from [2] for any 4-ended tangle in a  $\mathbb{Z}$ -homology 3-ball. This manual only describes how to use the main functionalities of this package. Help with more obscure functions included in `PQM.m` can be displayed in a notebook in the usual way by calling

`?ObscureFunction`

(which gives a description of `ObscureFunction`) or

`??ObscureFunction`

(for both a description and the actual definition). This manual should be read alongside the notebooks [3, 4, 6], where we compute the invariants for three basic examples. At the end of this manual, we showcase some outputs for these examples, see Figures 3, 5 and 6.

## 1. BASIC USAGE

**1.1. Input preparation.** The Mathematica package `PQM.m` implements the algorithm from [2, Corollary 5.7], which allows us to compute peculiar modules combinatorially from nice Heegaard diagrams. So, given a Heegaard diagram for a 4-ended tangle in a  $\mathbb{Z}$ -homology 3-ball, we first need to niceify it using Sarkar and Wang's nicefication algorithm from [1]. How we do this can have a significant impact on the run time of the computation for large diagrams, so one should keep the number of generators as low as possible. Once, we have a nice diagram, we label the intersection points of  $\alpha$ -curves and  $\beta$ -curves by integers  $(1, 2, 3, \dots)$ . Similarly, we label the regions in the Heegaard diagram  $(1, 2, 3, \dots)$ . Finally, we enumerate the  $\alpha$ -arcs and  $\alpha$ -curves and, separately, all  $\beta$ -curves. For examples, see Figures 2 and 4.

**1.2. Backups.** At any stage throughout the program, one can easily make backups of preliminary results via

```
DumpSave[BackupFilePath <> "_AfterCancellation.mx", "Global["];
```

For this, we need can specify a path `BackupFilePath` to the directory where the backups should be stored. They can then be recalled for example like this:

```
<< (BackupFilePath <> "_BeforeCancellation.mx");
```

---

*Date:* 8th April 2019.

1.3. **Input data.** We start by loading the package [5] as follows:

```
<< PQM.m
```

Next, we enter the following data into the notebook. For each calculation, a separate notebook should be used.

**regionsInput** is a matrix with five columns and a row for each region of the nice Heegaard diagram. The first entry of the  $i^{\text{th}}$  row should be equal to  $i$ . The other four entries of the  $i^{\text{th}}$  row are the vertices of the  $i^{\text{th}}$  region, ordered by their boundary orientation. Our orientation conventions are as in [Zib17]: The normal vector field, determined by the right hand rule, points into the plane, so the boundary orientation is clockwise. We start with a vertex which is the start of a segment of an  $\alpha$ -curve in the boundary of the region. For bigons, the last two entries remain empty, ie occupied by the symbol  $\square$ .

*Note:* The first column is not used anywhere in the program, it only helps a human being to translate between the picture of the Heegaard diagram and the Mathematica notebook.

**alphasInput** is a table whose rows are indexed by the  $\alpha$ -curves. Again, the first entry should be the index of the curve. The second is a list of all intersection points on this curve.

*Note:* The order of the intersection points is irrelevant.

**betasInput** is a table whose rows are indexed by the  $\beta$ -curves. Again, the first entry should be the index of the curve. The second is a list of all intersection points on this curve.

*Note:* The order of the intersection points is irrelevant.

**cancellationSortListInput** is a table of intersection points with two columns, so each row corresponds to a pair of intersection points. This table has an effect on the order of the generators and is important for the initial cancellation after computing the invariant. Usually, we start with a Heegaard diagram which is not necessarily nice and then niceify it using finger moves, thereby creating lots of new intersection points and generators. In the initial cancellation step, the program attempts to cancel such generators, thereby reversing the effect of niceification. The order in which this is done is determined by the order of the generators, and this, in turn, is determined by **cancellationSortListInput**. So the pairs of intersection points should be those that can be removed by a reversed finger move. The order of the intersection points for each pair is the same as for **regionsInput**, using the bigon which connects these two points and which is removed by the reversed finger move. This bigon accounts for the identity component in the differential which the program will attempt to cancel.

**alphaArcs** is a table whose four rows correspond to the four sites  $a$ ,  $b$ ,  $c$  and  $d$  of the tangle, as indicated by the entries of the first column. The second entry in each row is a list of all intersection points for the corresponding site.

*Note:* The first column should not be changed.

**basepointRegions** is a table with four columns. The entries of the first column are indices of regions containing the basepoint labelled by the corresponding entries of the second column, namely either  $p$  or  $q$ .

*Note 1:* Do not use any other variables; in particular, do not use  $p$  or  $q$  with subscripts such as  $p_1$  or  $q_4$ .

*Note 2:* In the very special case that there are multiple basepoints in this region, take a suitable power of  $p$  or  $q$ .

The third column corresponds to the Alexander grading; entries are lists of length equal to the number of colours in the tangle, such that the  $i^{\text{th}}$  entry of the list corresponds to the  $i^{\text{th}}$  colour. A basepoint of an open (closed) strand leaving/entering the 3-manifold should be recorded as  $+1/-1$  ( $+2/-2$ ) for the corresponding colour. The entries of the fourth column should be  $-2$  ( $-4$ ) for each basepoint of an open (closed) strand it contains. This information is used for the computation of the  $\delta$ -grading.

**multiplicity0Regions** is a table with four columns. The entries of the first column are indices of regions whose multiplicity in each domain is 0. The second entry is a list of oriented elementary  $\beta$ -segments (ie pairs of intersection points) along the boundary of the domain. The orientation conventions are as in **regionsInput**.

*Note:* Any  $\beta$ -segment which lies in the interior of the domain should be recorded once in each direction.

The third column corresponds to the Alexander grading; entries are lists of length equal to the number of colours in the tangle, such that the  $i^{\text{th}}$  entry of the list corresponds to the  $i^{\text{th}}$  colour. A basepoint of an open (closed) strand leaving/entering the 3-manifold should be recorded as  $+1/-1$  ( $+2/-2$ ) for the corresponding colour. The entries of the fourth column should be  $4 \cdot (\text{Euler measure of region})$  plus  $-2$  ( $-4$ ) for each basepoint of an open (closed) strand it contains. This information is used for the computation of the  $\delta$ -grading.

**1.4. Verifying the input data.** Before we start the actual calculation, we should make sure that the input data that we have entered is consistent and does indeed correspond to our Heegaard diagram. At the end of the cell containing the basic input data above, we call **Step1Preparation**. This returns a list of results of automated sanity checks and some additional outputs, which one should check manually. It returns the total number of nice regions (**NR**), the number of intersection points between  $\alpha$ - and  $\beta$ -curves (**NI**). It also prints lists named **0 vertices**, **+1 vertices**, etc, which partition the set of intersection points into five subsets as follows. An intersection point is in **<n> vertices** if the sum of unlabelled regions (ie those adjacent to basepoints) in the four quadrants around it equals  $n$ , where each region contributes as follows: Walking around an intersection point in anticlockwise direction, an unlabelled region that we enter through a  $\beta$ -curve counts as  $+1$ , one that we exit through a  $\beta$ -curve as  $-1$ .

**1.5. Running a calculation.** Once we have convinced ourselves that the input data is correct, we run the program in several separate steps by evaluating

```

Step2Generators,
Step3Domains,
Step4Gradings,
Step5Differentialsand
Step6Cancellation.

```

Like `Step1Preparation`, these are modules defined in the package [5] which group together blocks of code that compute the various components of the invariant. Each step might give some further feedback, such as the number of generators in each site or the number of domains. Unless there are error messages, one may safely ignore these messages.

1.6. **Cancellation.** After calling `Step6Cancellation`, we run

```
CancellationData = Cancellation[differentials, generators, 1];
```

The `CancellationData` is a list of two elements, the first of which contains the data for the differentials of the peculiar module after cancellation and the second contains the data for the generators of the peculiar module after cancellation.

1.7. **Post-Processing.** We finally run `Step7PostProcessing`. This loads tools for displaying peculiar modules graphically and for finding the corresponding immersed curve invariants.

`GenTableWithIdems[gens]` displays a list of generators `gens`, ordered by idempotents.

`DSquared0Q[maps]` verifies if the differential `maps` satisfies the relation  $d^2 = 0$ . `ShowGraph[maps, gens, VertexLabelSwitch:1, EdgeLabelSwitch:1, pos:0, CoordList:Automatic]` draws a graphical representation of `maps`. `gens` is the underlying set of generators with differentials `maps`.

- (1) The optional parameter `VertexLabelSwitch` can be set to 0 to suppress any labelling of vertices, 1 (default) to show the generator index or 2 to give full details on generators.
- (2) The optional parameter `EdgeLabelSwitch` can be set to 0 to suppress any labelling and orientation of edges or 1 (default) to show both. Note that the edges are dashed iff they correspond to differentials along powers of  $q$ ; this agrees with the conventions in [2].
- (3) The optional parameter `pos` is an integer by default, in which case all generators are shown; alternatively, `pos` can be a list of indices of generators in `gens`, in which case only the full subgraph spanned by these generators is shown.
- (4) Finally, the optional parameter `CoordList` can be set to a list of coordinates for all vertices of the displayed graph. If no such coordinate list is specified, `SpringElectricalEmbedding` is chosen as the preferred style.

`DotGrid[gens, subset:0, alexstart:3]` displays the generators and their gradings; the first two Alexander gradings (usually those for the two open strands) are shown graphically in terms of their position in a grid:  $t_1$  increases from top to bottom in steps of  $\frac{1}{2}$ ,  $t_2$  increases from left to right in steps of  $\frac{1}{2}$ . The generators are shown as dots whose colour corresponds to the four sites of the tangle. The index of the generator is shown in the

dot. A label above the generator shows the  $\delta$ -grading along with any other Alexander gradings. `DotGrid` takes three optional parameters:

- (1) The first can be used to display only a subset of generators, by specifying a list of corresponding generator indices.
- (2) The second parameter can be used to vary the number of Alexander gradings. Usual values are
  - (a) 0 (show no Alexander gradings),
  - (b) 1 (show all Alexander gradings),
  - (c) 3 (default: show all Alexander gradings except the first two),
  - (d) -1 (collapse all Alexander gradings),
  - (e) a list of  $\pm 1$ s as in `CollapseAlexGradings` to reverse some orientations before collapsing.
- (3) The third parameter can be used to show generators in the same gradings as distinct dots labelled by their indices (0: default), or as single dots with multiplicities without any indices (1).

`SimplifyPQM[maps,MaxIterations:200]` performs a sequence of homotopies by alternately simplifying the complex with respect to the variables  $p$  and  $q$ , using the function `SeparateAllDifferentials`. The iteration terminates either if the complex becomes loop-type (see: `CheckIfLoopType`), or after `MaxIterations` iterations. Since a pseudo-random function is invoked by `SeparateAllDifferentials`, the number of iterations to put a complex in loop-type position might vary, as well as the output, if the complex is not in loop-type position.

`ShowResult[maps, gens, switch:'all']` displays the generators arranged as in `DotGrid` for each supported Alexander grading corresponding to the colours of closed components along with the complex, sorted into connected components. The complex can be suppressed by setting the third optional parameter to `gens`.

## 2. EXAMPLES

In [2, section 6.3], the peculiar modules of the  $(2n, -(2m + 1))$ -pretzel tangles from Figure 1 are computed for all  $n, m > 0$ . We can now use `PQM.m` to easily confirm these calculations for fixed  $n$  and  $m$ .

**Example 2.1**  $((6, -9)$ -pretzel tangle;  $n = 3, m = 4$ ). A nice Heegaard diagram for the  $(6, -9)$ -pretzel tangle is shown in Figure 3, which is a special case of the Heegaard diagram from [2, Figure 53a]. Figure 2 shows the output of the program from the notebook [4]: on the top, we see the simplified peculiar module, the lower part shows its generators with their gradings. To display the generator indices, one can change some parameters of `DotGrid` and `ShowGraph`, or simply use `ShowResult`. This is an example of the case  $n \leq m + 1$  in [2, Figure 52].

**Example 2.2**  $((10, -5)$ -pretzel tangle;  $n = 5, m = 2$ ). A nicefied Heegaard diagram for the  $(10, -5)$ -pretzel tangle is shown in Figure 4. The calculation is done in the notebook [3]. The top part of Figure 5 shows the simplified peculiar module,

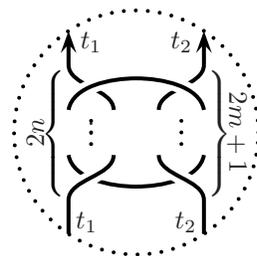

FIGURE 1. The pretzel tangle from Examples 2.1 and 2.2.

the lower part the generators of this module with their gradings. This is an example of the case  $n > m + 1$  in [2, Figure 52].

Finally, let us include one more example for which we do not already know the invariant.

**Example 2.3** ( $(2, -2)$ -pretzel tangle). Figure 6 shows the simplified peculiar module for the  $(2, -2)$ -pretzel tangle, which is the trivial tangle with one unknot component winding around both strands.

#### REFERENCES

- [1] S. Sarkar and J. Wang. An algorithm for computing some Heegaard Floer homologies. *Ann. of Math. (2)*, 171(2):1213–1236, 2010. (arXiv:math/0607777v4).
- [2] C. B. Zibrowius. Peculiar modules for 4-ended tangles. *arXiv preprint*, 2017. (arXiv:1712.05050v2).
- [3] C. B. Zibrowius. `10m5pt.nb`, 2019. Mathematica notebook, ancillary file to (arXiv:1712.05050v2).
- [4] C. B. Zibrowius. `6m9pt.nb`, 2019. Mathematica notebook, ancillary file to (arXiv:1712.05050v2).
- [5] C. B. Zibrowius. `PQM.m`, 2019. Mathematica package, ancillary file to (arXiv:1712.05050v2).
- [6] C. B. Zibrowius. `TrivialPlus1.nb`, 2019. Mathematica notebook, ancillary file to (arXiv:1712.05050v2).

*E-mail address:* `claudius.zibrowius@posteo.net`

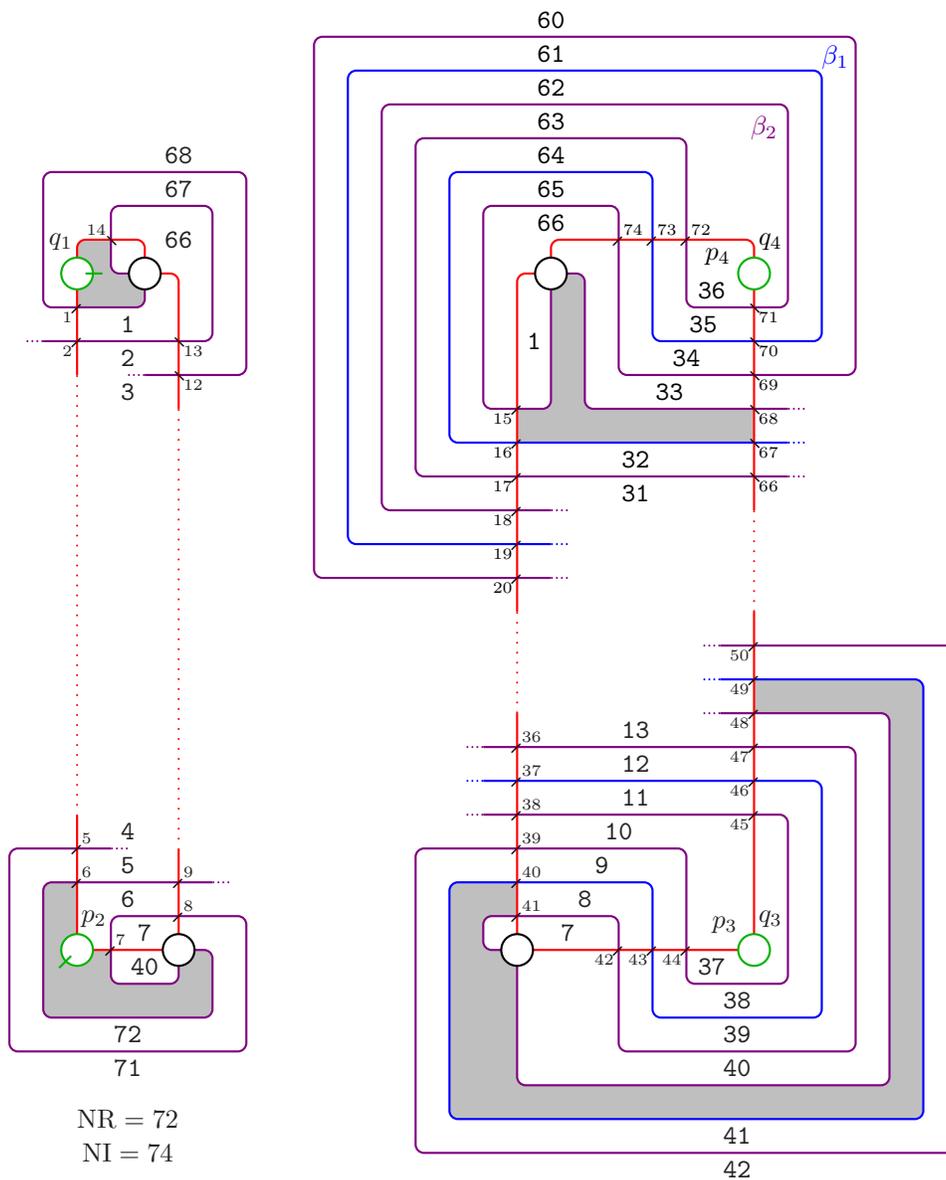

FIGURE 2. The Heegaard diagram for the  $(6, -9)$ -pretzel tangle from example 2.1.



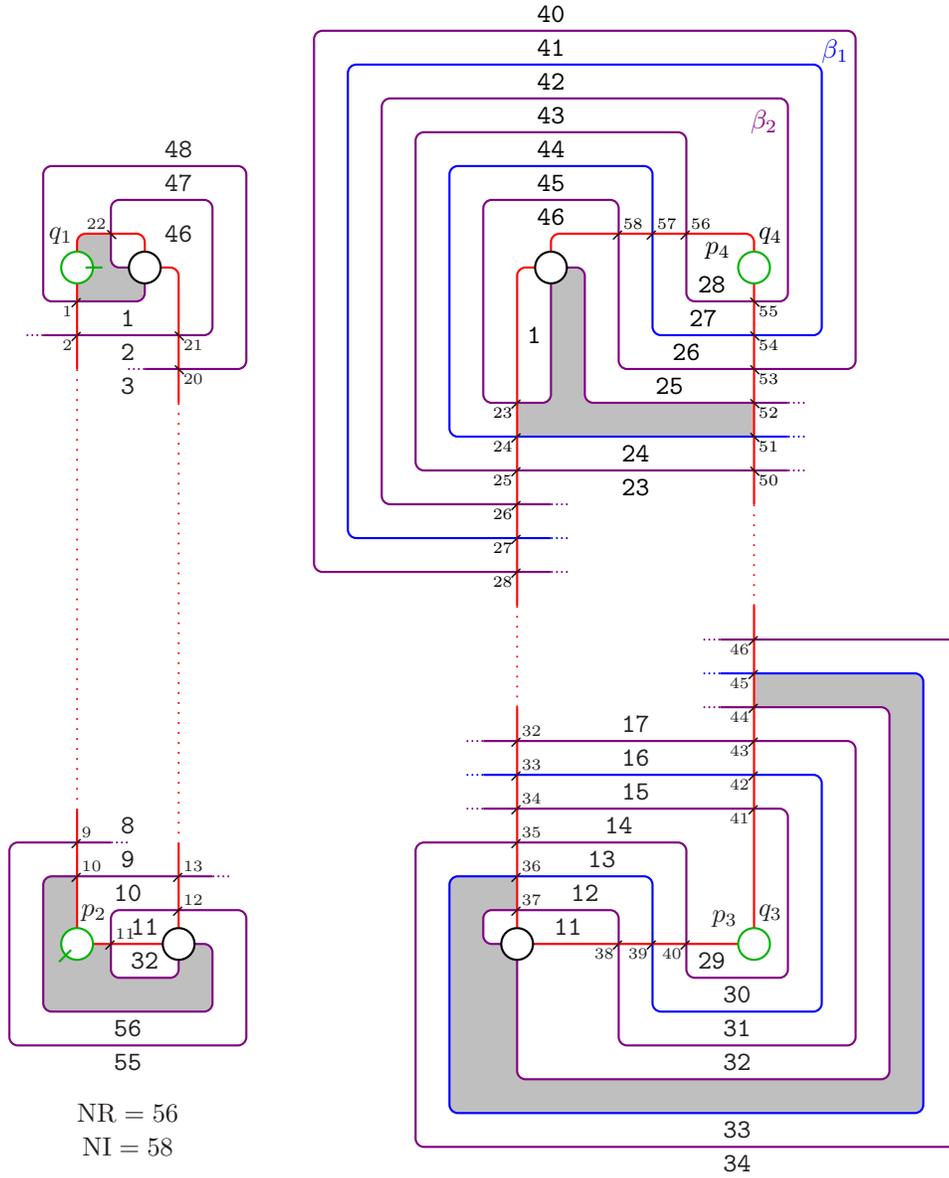

FIGURE 4. *The Heegaard diagram for the  $(10, -5)$ -pretzel tangle from example 2.2.*



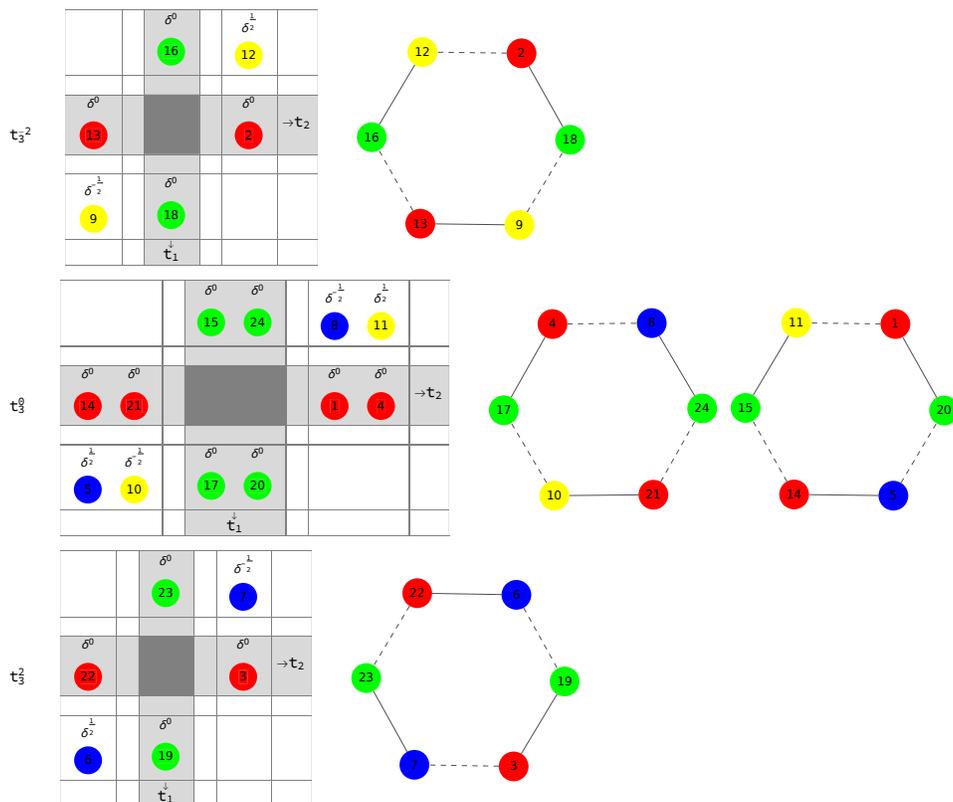

FIGURE 6. The output of `ShowResult[DD2, GG1, "all"]` for the  $(2, -2)$ -pretzel tangle (example 2.3) from [6].
